# Supplementary material for: Pointwise Mutual Information Based Metric and Decoding Strategy for Faithful Generation in Document Grounded Dialogs
Source: arXiv:2305.12191 source file (2023-12-01)
Supplement: Supplementary file 1 [file appendix_ablation.tex]

% \begin{table}[ht]
\begin{table}
\centering
%\small
% \resizebox{\columnwidth}{!}{
\begin{tabular}{ll|ll|ll}
\toprule
& & \multicolumn{2}{|c|}{\textbf{PMIF (Document)}} & \multicolumn{2}{|c}{\textbf{RougeL (Gold)}}\\
& & $top\ p$ & & $top\ p$ &\\
Dataset & $\alpha$ & 0.6 & 1.0 & 0.6 & 1.0  \\
\midrule
\multirow{4}{*}{\shortstack{Multi-\\Doc2Dial}} & 0.0 & 1.71& 1.71 &	0.49 &	0.49\\
& 0.25 &	1.73 &	1.95 &	0.40 &	0.39\\
& 0.5 &	1.76 & 2.03 &	0.39 &	0.34\\
& 1.0 &	1.70 & 0.37 &	0.37 &	0.10\\
\midrule
\multirow{4}{*}{\shortstack{Topical\\Chat}} & 0.0 &	1.05 &	1.05 &	0.22 &	0.22\\
& 0.25 &	1.44 &	1.60 &	0.20 &	0.20\\
& 0.5 &	1.55 &	1.83 &	0.19 &	0.15\\
& 1.0 &	1.53 &	0.25 &	0.17 &	0.02\\
\midrule
\multirow{4}{*}{\shortstack{Faith\\Dial}} & 0.0 &	1.36 &	1.36 &	0.40 &	0.40\\
& 0.25 &	1.73 &	1.95 &	0.40 &	0.39\\
& 0.5 &	1.76 &	2.03 &	0.39 &	0.34\\
& 1	& 1.70 &	0.37 &	0.37 &	0.10\\
\bottomrule
\end{tabular}
% }
\caption{\label{tab:ablation}}
\end{table}
